# Supplementary material for: Fast Green's function method for ultrafast electron-boson dynamics
Source: arXiv:2006.14965 source file (2021-03-29)
Supplement: Supplementary file 1 [file SupplementaryMaterials.pdf]

# Supplementary Material for "Fast Green's function method for ultrafast electron-boson dynamics"

## I. DERIVATION OF THE ELECTRON-BOSON GKBA

The form of the bosonic GKBA can be derived using properties for the non-interacting propagators. For the discussion, we need the explicit form of the lesser and greater non-interacting Green's functions, as well as the retarded and advanced ones.

Let us consider non-interacting bosons under the influence of a time-dependent Hamiltonian $\Omega(t)$. Let us take the initial state as a thermal state with inverse temperature $\beta$. In the uncorrelated case, where the bosonic self-energy $\boldsymbol{\Pi} = 0$, the (fluctuation) lesser and greater bosonic Green's function is given as a solution of the non-interacting bosonic KBE[1]

$$\boldsymbol{d}^{\lessgtr}(t,t') = -i\boldsymbol{\alpha}\boldsymbol{V}(t) f^{\lessgtr}(\beta\bar{\boldsymbol{\Omega}}^{M}\boldsymbol{\alpha})\boldsymbol{V}^{-1}(t'), \tag{1}$$

where $f^{>}(\omega) = 1 + f^{<}(\omega)$ and $f^{<}(\omega) = \frac{1}{\mathrm{e}^{\omega}-1}$ is the Bose function, and the non-unitary operator $\boldsymbol{V}(t)$ is

$$\boldsymbol{V}(t) = \mathcal{T}\left\{ \mathrm{e}^{-i\int_{t_0}^{t} \mathrm{d}\bar{t}\, \bar{\boldsymbol{\Omega}}(\bar{t})\boldsymbol{\alpha}} \right\}. \tag{2}$$

The bosonic density matrix $\boldsymbol{\rho}_{\mathrm{b}}(t) \equiv \boldsymbol{\rho}^{<}_{\mathrm{b}}(t)$ is given by $\boldsymbol{\rho}_{\mathrm{b}}(t) = i\boldsymbol{d}^{<}(t,t)$, and the initial density matrix is then given by $\boldsymbol{\rho}_{\mathrm{b}}(t_0) = \boldsymbol{\alpha} f^{<}(\beta\bar{\boldsymbol{\Omega}}(t_0)\boldsymbol{\alpha})$.

The explicit expressions of the real-time lesser and greater functions yields the retarded and advanced functions as

$$\boldsymbol{d}^{R/A}(t,t') = \mp i\boldsymbol{\alpha}\theta\left[\pm(t-t')\right]\boldsymbol{V}(t)\boldsymbol{V}^{-1}(t') \tag{3}$$

The above equations can be used for deriving the bosonic GKBA by finding an equivalent form of the non-interacting equation, Eq. (1). Let us consider $t > t'$, and insert the relation $\hat{\mathbb{1}} = \boldsymbol{V}^{-1}(t')\boldsymbol{V}(t')$ between $\boldsymbol{V}(t)$ and $f^{\lessgtr}(\beta\bar{\boldsymbol{\Omega}}(t_0)\boldsymbol{\alpha})$ in Eq. (1). This yields

$$\boldsymbol{d}^{\lessgtr}(t;t') = \boldsymbol{d}^{R}(t,t')\boldsymbol{\alpha}\boldsymbol{\rho}^{\lessgtr}_{\mathrm{b}}(t'), \quad \text{for } t > t'. \tag{4}$$

We can treat the case $t' > t$ similarly, and the full expression, valid for all $t$ and $t'$, becomes

$$\boldsymbol{d}^{\lessgtr}(t,t') = \boldsymbol{d}^{R}(t,t')\boldsymbol{\alpha}\boldsymbol{\rho}^{\lessgtr}_{\mathrm{b}}(t') - \boldsymbol{\rho}^{\lessgtr}_{\mathrm{b}}(t)\boldsymbol{\alpha}\boldsymbol{d}^{A}(t,t'). \tag{5}$$

The resulting expression for $\boldsymbol{d}^{\lessgtr}(t,t')$, Eq. (5), is equivalent to Eq. (1) for the non-interacting case. However, by promoting the density matrix $\boldsymbol{\rho}^{\lessgtr}_{\mathrm{b}}$ to be a correlated one, the two expressions differ. Inserted into the collision integrals, Eq. (5) represents a non-trivial Ansatz for the lesser and greater Green's functions. As such, we refer to Eq. (5), with a correlated density matrix, as the bosonic GKBA.

## II. SELF-ENERGIES

In this work, we consider the $GD$ approximation, in which we retain the lowest order diagrams in terms of the bosonic propagator. The explicit shape of the self-energies are given by[1–3]

$$\Sigma^{\lessgtr}_{pq}(t,t') = i\sum_{\bar{\mu}\bar{\nu}rs} \lambda^{\bar{\mu}}_{pr}(t) D^{\lessgtr}_{\bar{\mu}\bar{\nu}}(t,t')\lambda^{\bar{\nu}}_{sq}(t') G^{\lessgtr}_{rs}(t,t'), \tag{6}$$

$$\Pi^{\lessgtr}_{\bar{\mu}\bar{\nu}}(t,t') = -i\sum_{pqsr} \lambda^{\bar{\mu}}_{pq}(t) G^{\lessgtr}_{qs}(t,t') G^{\gtrless}_{rp}(t',t)\lambda^{\bar{\nu}}_{sr}(t'). \tag{7}$$

These self-energies can be generated from a generating $\Phi[G,\boldsymbol{D}]$ functional via

$$\Sigma[G,\boldsymbol{D}] = \frac{\delta\Phi}{\delta G}, \qquad \boldsymbol{\Pi}[G,\boldsymbol{D}] = -2\left.\frac{\delta\Phi}{\delta\boldsymbol{D}}\right|_{S}, \tag{8}$$

where the equation for $\boldsymbol{\Pi}$ contains a symmetrized functional derivative, indicated by subscript $S$[1–3].

## III. CONSERVING PROPERTIES OF THE ELECTRON-BOSON GKBA

A conserving approximation yields observables that satisfies conservation laws, such as the conservation of particle number, momentum, angular momentum, and energy. In this section, we show that the GKBA is part of a more general structure of conserving approximations.

A straightforward way to see if a given diagrammatic approximation is conserving is to make use of a generating functional $\Phi[G,\boldsymbol{D}]$[4], which is a functional of $G$ and $\boldsymbol{D}$, two-point functions on the Keldysh contour $\gamma$[5]. If we construct the contour self-energies $\Sigma$ and $\boldsymbol{\Pi}$ via a functional derivative as in Eq. (8), and use the functionals $\Sigma[G,\boldsymbol{D}]$ and $\boldsymbol{\Pi}[G,\boldsymbol{D}]$ in the KBE, solved self-consistently, the resulting scheme is conserving provided that the generating functional $\Phi$ satisfies certain symmetries[4–6]. Gauge symmetry, for example, yields particle number conservation[4].

For the GKBA approximate scheme, the above considerations have to be slightly modified. The reason is that the GKBA scheme only applies to the time-diagonal part. A consistent extension of the GKBA scheme to the off-diagonal time part[7], yields equations of motion with a different structure than the usual KBE, namely

$$\left[i\partial_z - \hat{h}(z)\right]\hat{\mathcal{G}}(z,z') = \int_{\gamma} \mathrm{d}\bar{z}\, \hat{\Sigma}_A(z,\bar{z})\hat{\mathcal{G}}_A(\bar{z},z'),$$
$$\left[i\partial_z - \boldsymbol{\alpha}\bar{\boldsymbol{\Omega}}\right]\boldsymbol{D}(z,z') = \boldsymbol{\alpha}\int_{\gamma} \mathrm{d}\bar{z}\, \boldsymbol{\Pi}_A(z,\bar{z})\boldsymbol{D}_A(\bar{z},z'), \tag{9}$$

together with their corresponding adjoint equations. In Eq. (9), $A$ stands for an auxiliary Green's function, and for notational simplicity we write $\Sigma_A = \Sigma[G_A,\boldsymbol{D}_A]$, and similar for $\boldsymbol{\Pi}_A$. The variables $z, z'$ are times on the Keldysh contour. In the case of the GKBA, the equation for the density matrices $\rho$ and $\boldsymbol{\rho}_{\mathrm{b}}$

can be obtained by subtracting the corresponding KBE and its adjoint, using the Langreth rules[5] to obtain real-time equations, and then inserting the EB GKBA in place of the auxiliary Green's functions.

Despite the different structure from the KBE, solving the above equation, Eq. (9), with the collision integral coming from a generating functional $\Phi$, still fulfills the same conservation laws. As has also been noted in Ref. 8 regarding one-shot Green's function calculations, with such a structure the same procedure from Baym[4] can be carried out. As such, equations having the structure of Eq. (9) are conserving under the same conditions as for the KBE; in particular the GKBA. We demonstrate the procedure for two conservation laws: Particle number conservation, and energy conservation. We refer to Ref. 9 for a discussion on momentum conservation.

The conservation laws are given by specific variations of $\Phi$ when varying the two-point functions $\boldsymbol{G}$ and $\boldsymbol{D}$, denoted by $\delta\boldsymbol{G}$ and $\delta\boldsymbol{D}$ respectively. Symbolically, we have, by definition,

$$\delta\Phi = \int \Sigma\,\delta\boldsymbol{G} - \frac{1}{2}\int \boldsymbol{\Pi}\,\delta\boldsymbol{D}, \tag{10}$$

with $\delta\Phi = \Phi[\boldsymbol{G}+\delta\boldsymbol{G}, \boldsymbol{D}+\delta\boldsymbol{D}] - \Phi[\boldsymbol{G}, \boldsymbol{D}]$. We stress that the variations are made for *general* two-point functions $\boldsymbol{G}$ and $\boldsymbol{D}$.

### A. Particle number conservation

Particle conservation is most conveniently discussed in real space. We denote the space-spin variable $\mathbf{x}_1 = (r_1, \sigma_1)$, and $1 = (\mathbf{x}_1, z_1)$. From the electronic KBE-like structure of Eq. (9), taking the $z' = z^+$, $\mathbf{x}' = \mathbf{x}$ limit and subtracting the equations yield the contour *continuity equation*[3,5]

$$\frac{\mathrm{d}}{\mathrm{d}z_1} n(1) + \nabla\cdot\mathbf{j}(1) = \\ = -\int_\gamma \mathrm{d}3 \left[\Sigma_A(1,3)\boldsymbol{G}_A(3,1^+) - \boldsymbol{G}_A(1,3)\Sigma_A(3,1^+)\right] \tag{11}$$

where $n(1)$ is the particle density and $\mathbf{j}(1)$ is the current density. The right-hand side of Eq. (11) is an unphysical source/drain term, which can be non-zero for non-conserving approximations, violating particle number conservation.

If the generating functional $\Phi[\boldsymbol{G}, \boldsymbol{D}]$ has the symmetry $\Phi[\boldsymbol{G}, \boldsymbol{D}] = \Phi[\mathrm{e}^{i\Lambda}\boldsymbol{G}\mathrm{e}^{-i\Lambda}, \boldsymbol{D}]$, a symmetry guaranteed if $\Phi$ consists of closed electron loops[3], for infinitesimal $\Lambda$ one obtains from Eq. (10), with $\delta\boldsymbol{D} = 0$,

$$0 = \int_\gamma \mathrm{d}3 \left[\Sigma(1,3)G(3,1^+) - G(1,3)\Sigma(3,1^+)\right], \tag{12}$$

where we write $\Sigma = \Sigma[\boldsymbol{G}, \boldsymbol{D}]$. Thus, the right-hand side of Eq. (12) equals zero, a property which we stress is valid for all two-point functions $\boldsymbol{G}$ and $\boldsymbol{D}$. In particular, evaluating the two-point functions at $\boldsymbol{G}_A$ and $\boldsymbol{D}_A$, the right-hand side of Eq. (12) is precisely the source/drain in Eq. (11). Inserting the EB GKBA we find that the EB GKBA scheme fulfills electronic (not bosonic) particle conservation.

### B. Formula for the total energy

For simplicity, we do not consider an electronic two-body interaction here. The total energy of the system is then given by

$$E(z) = E_{\mathrm{el}}(z) + E_{\mathrm{bos}}(z) + E_{\mathrm{MF}}(z) + E_c(z), \tag{13}$$

where the electronic single-particle energy is

$$E_{\mathrm{el}}(z) = \mathrm{Tr}_e[h(z)\rho(z)], \tag{14}$$

the bosonic single-particle energy is

$$E_{\mathrm{bos}}(z) = \mathrm{Tr}_b[\Omega(\rho_{\mathrm{b}}(z) + \boldsymbol{\phi}(z)\otimes\boldsymbol{\phi}(z))], \tag{15}$$

the mean-field energy is

$$E_{\mathrm{MF}}(z) = \mathrm{Tr}_e[h_{\mathrm{bos}}(z)\rho(z)], \tag{16}$$

and $E_c$ is the correlation energy. The symbols $\mathrm{Tr}_e$ and $\mathrm{Tr}_b$ refers to electronic and bosonic trace, respectively. The exact EB correlation energy $E_c(z)$ is given by

$$E_c(z) = \sum_{pq\bar{\mu}} \lambda^{\bar{\mu}}_{pq} \left\langle \Delta\hat{\phi}_{H,\bar{\mu}}(z)\hat{c}^\dagger_{H,p}(z)\hat{c}_{H,q}(z)\right\rangle, \tag{17}$$

and can be equivalently be written in terms of the electronic or the bosonic collision integrals, as

$$\begin{aligned} E_c^{(1)}(z) &= -i\int_\gamma \mathrm{d}\bar{z}\,\mathrm{Tr}_e\left[\Sigma_A(z,\bar{z})\boldsymbol{G}_A(\bar{z},z^+)\right], \\ E_c^{(2)}(z) &= i\int_\gamma \mathrm{d}\bar{z}\,\mathrm{Tr}_b\left[\boldsymbol{\Pi}_A(z,\bar{z})\boldsymbol{D}_A(\bar{z},z^+)\right]. \end{aligned} \tag{18}$$

The two expressions for the correlation energy are identical for the *exact* case, $E_c^{(1)}(z) = E_c^{(2)}(z)$. A given diagrammatic approximation, however, is not guaranteed to satisfy these conditions; a simple example being the $\boldsymbol{Gd}$ approximation for which $E_c^{(2)}(z) = 0$, but $E_c^{(1)}(z) \neq 0$.

In a given diagrammatic approximation, the expressions for the correlation energy in Eq. (18) can be rewritten, using (omitting contour-time arguments)

$$\int_\gamma \mathrm{Tr}_e\left[\Sigma_A\boldsymbol{G}_A\right] = \int_\gamma \mathrm{Tr}_e\left[\boldsymbol{G}_A\Sigma_A\right], \tag{19}$$

valid if the continuity equation is satisfied in the approximation, and

$$\int_\gamma \mathrm{Tr}_b\left[\boldsymbol{\Pi}_A\boldsymbol{D}_A\right] = \int_\gamma \mathrm{Tr}_b\left[\boldsymbol{D}_A\boldsymbol{\Pi}_A\right], \tag{20}$$

valid due to the symmetry $\boldsymbol{D}_{\bar{\mu}\bar{\nu}}(z,z') = \boldsymbol{D}_{\bar{\nu}\bar{\mu}}(z',z)$ and the same for $\boldsymbol{\Pi}$. As such, we obtain the following expressions for the correlation energies:

$$\begin{aligned} E_c^{(1)}(z) &= -\frac{i}{2}\int_\gamma \mathrm{Tr}_e\left[\Sigma_A\boldsymbol{G}_A + \boldsymbol{G}_A\Sigma_A\right], \\ E_c^{(2)}(z) &= \frac{i}{2}\int_\gamma \mathrm{Tr}_b\left[\boldsymbol{\Pi}_A\boldsymbol{D}_A + \boldsymbol{D}_A\boldsymbol{\Pi}_A\right]. \end{aligned} \tag{21}$$

In the EB GKBA, from the symmetrized expressions Eq. (21), we can obtain the correlation energy as

$$
\begin{aligned}
E_c^{(1)}(t) &= -\frac{i}{2}\mathrm{Tr}_e\left[\boldsymbol{I}(t) - \boldsymbol{I}^\dagger(t)\right],\\
E_c^{(2)}(t) &= \frac{i}{2}\mathrm{Tr}_b\left[\boldsymbol{\alpha}\boldsymbol{I}_b(t) + (\boldsymbol{\alpha}\boldsymbol{I}_b(t))^T\right].
\end{aligned}
\tag{22}
$$

It is straightforward to show that, in the $\boldsymbol{GD}$ approximation in our EB GKBA scheme, the two expressions are identical.

### C. Energy conservation from varying the functional

Energy conservation for $\Phi$-derivable schemes is connected to the following variation of $\boldsymbol{G}$ and $\boldsymbol{D}$[6]:

$$
\begin{aligned}
\boldsymbol{G} &\rightarrow \left(\frac{\mathrm{d}w(z_1)}{\mathrm{d}z_1}\right)^{\frac{1}{4}} \boldsymbol{G}_{pq}(w(z_1); w(z_2)) \left(\frac{\mathrm{d}w(z_2)}{\mathrm{d}z_2}\right)^{\frac{1}{4}},\\
\boldsymbol{D} &\rightarrow \left(\frac{\mathrm{d}w(z_1)}{\mathrm{d}z_1}\right)^{\frac{1}{2}} \boldsymbol{D}_{\bar{\mu}\bar{\nu}}(w(z_1); w(z_2)) \left(\frac{\mathrm{d}w(z_2)}{\mathrm{d}z_2}\right)^{\frac{1}{2}},
\end{aligned}
\tag{23}
$$

where $w$ is an invertible mapping on the contour. For these variations, $\delta\Phi = 0$, and from Eq. (10) we obtain, for infinitesimal $w$, $0 = \delta_{\boldsymbol{G}}[\boldsymbol{G}, \boldsymbol{D}](z) + \delta_{\boldsymbol{D}}[\boldsymbol{G}, \boldsymbol{D}](z)$, with

$$
\begin{aligned}
\delta_{G} = \int_\gamma \mathrm{d}\bar{z}\, \mathrm{Tr}_e \Big\{ &-\frac{1}{4}\partial_{z_1}\left[\Sigma(z;\bar{z})\boldsymbol{G}(\bar{z}; z^+) + \boldsymbol{G}(z_1;\bar{z})\Sigma(\bar{z}, z^+)\right]\\
&+ \left[\Sigma(z;\bar{z})\left(\partial_z \boldsymbol{G}(\bar{z}, z^+)\right) + \left(\partial_z \boldsymbol{G}(z;\bar{z})\right)\Sigma(\bar{z}, z^+)\right]\Big\},
\end{aligned}
$$

and

$$
\begin{aligned}
\delta_{\boldsymbol{D}} = \int_\gamma \mathrm{d}\bar{z}\, \mathrm{Tr}_B \Big\{ &\frac{1}{4}\partial_z\left[\boldsymbol{D}(z,\bar{z})\boldsymbol{\Pi}(\bar{z}, z^+) + \boldsymbol{\Pi}(z,\bar{z})\boldsymbol{D}(\bar{z}, z^+)\right]\\
&-\frac{1}{2}\left[\left(\partial_z \boldsymbol{D}(z,\bar{z})\right)\boldsymbol{\Pi}(\bar{z}, z^+) + \boldsymbol{\Pi}(z,\bar{z})\left(\partial_z \boldsymbol{D}(\bar{z}, z^+)\right)\right]\Big\},
\end{aligned}
$$

where we introduced the corresponding electronic and bosonic trace. We again stress that the equation $0 = \delta_{\boldsymbol{G}}[\boldsymbol{G}, \boldsymbol{D}] + \delta_{\boldsymbol{D}}[\boldsymbol{G}, \boldsymbol{D}]$ is satisfied for *any* two-point functions $\boldsymbol{G}$, $\boldsymbol{D}$.

The terms in $0 = \delta_{\boldsymbol{G}} + \delta_{\boldsymbol{D}}$ are related to time derivatives of different energy contributions. In an approximation where $E_c^{(1)}(z) = E_c^{(2)}(z)$, we can use the symmetrized version, Eq. (21), to equivalently write the correlation energy as $E_c(z) = \frac{1}{2}(E_c^{(1)}(z) + E_c^{(2)}(z))$. The time derivative $\frac{\mathrm{d}}{\mathrm{d}z}E_c(z)$ yields precisely the first two terms in $\delta_{\boldsymbol{G}}$, and the first two terms in $\delta_{\boldsymbol{D}}$, if we evaluate $\boldsymbol{G}$ and $\boldsymbol{D}$ in $\boldsymbol{G}_A$ and $\boldsymbol{D}_A$. The remaining terms from the variation of the $\Phi$-functional can be related to the time derivatives of the single-particle energies using the same arguments as in Refs. 5 and 6, ensuring the conservation of energy.

## IV. NUMERICAL EXAMPLE: HOLSTEIN DIMER

The Holstein model is a hallmark of strongly-correlated EB systems and a textbook example to discuss the formation of polarons[10]. Here, we use the Holstein dimer to benchmark the EB GKBA and demonstrate the conservation of energy. The Holstein dimer is described by the Hamiltonian

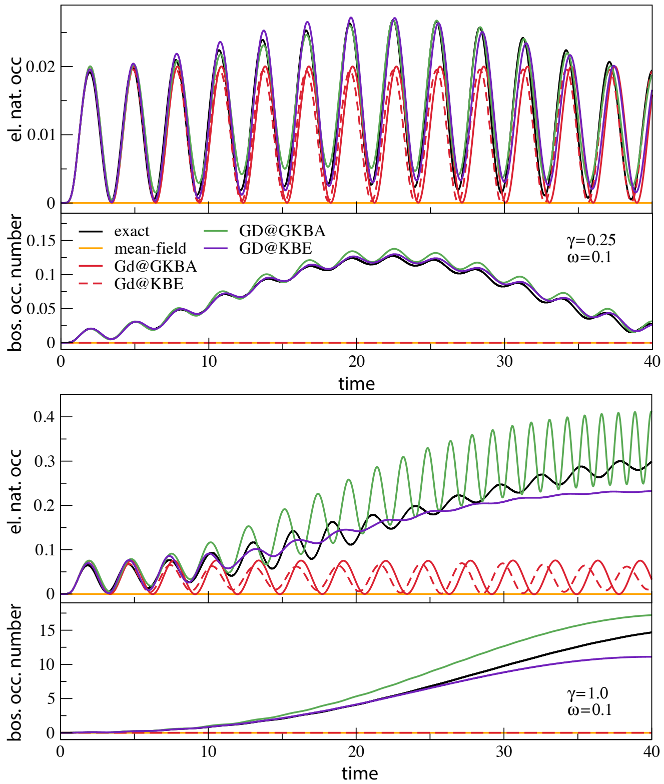


FIG. 1. Benchmark of Eq. (24), with intermediate interaction strength $\gamma = g^2/(\omega T) = 0.25$ (upper) and strong interaction strength $\gamma = 1.0$ (lower), with the interaction suddenly switched on at $t = 0$.

$$
\hat{H}(t) = -T(\hat{c}_1^\dagger \hat{c}_2 + \hat{c}_2^\dagger \hat{c}_1) + \omega \hat{a}^\dagger \hat{a} - \sqrt{2}g(t)\hat{\phi}_1(\hat{n}_1 - \hat{n}_2), \tag{24}
$$

where $\hat{n}_i = \hat{c}_i^\dagger \hat{c}_i$ is the electron number operator for spinless electrons on site $i$. The EB interaction couples a single bosonic mode to the electronic dipole operator, proportional to $\hat{n}_1 - \hat{n}_2$. In our notations in the main text, $h_{\mathrm{HF},12} = h_{\mathrm{HF},21} = -T$, $h_{\mathrm{HF},11} = h_{\mathrm{HF},22} = 0$, $\lambda^{\xi}_{pq}(t) = \delta_{\xi 1}\delta_{pq}(-\delta_{p1} + \delta_{p2})\sqrt{2}g(t)$, and $\boldsymbol{\Omega} = \frac{\omega}{2}\begin{pmatrix} 1 & i \\ -i & 1 \end{pmatrix}$. We choose $T = 1$ as our energy unit, $\omega = 0.1$ and the initial state as the non-interacting ground state, hence $\rho(0) = \frac{1}{2}\begin{pmatrix} 1 & 1 \\ 1 & 1 \end{pmatrix}$, $\rho_\mathrm{b}(0) = \frac{1}{2}\begin{pmatrix} 1 & -i \\ i & 1 \end{pmatrix}$. The EB interaction is switched on abruptly with the protocol $g(t) = g\left(\theta(T_s - t)\sin^2\left(\frac{\pi t}{2T_s}\right) + \theta(t - T_s)\right)$ with switching time $T_s = 1.0$. Since the Hamiltonian is invariant under the canonical transformation $\hat{c}_1 \leftrightarrow \hat{c}_2$ and $\hat{a} \rightarrow -\hat{a}$[2], the density remains homogeneous during the time evolution. This implies that $\phi_{1,2}(t) = 0$ and hence the mean-field term $h_{\mathrm{bos}}(t)$ vanishes; the dynamics is driven only by correlations.

### A. Populations

We compare the EB GKBA dynamics to exact results, obtained from the open-source computer package QuSpin[11,12], and to KBE simulations[13]. In Fig. 1 we show the lowest electronic natural occupation number (lowest eigenvalue of $\rho(t)$) as well as the number of bosons $\langle \hat{a}^\dagger \hat{a}\rangle(t)$ given by

$$\langle \hat{a}^\dagger_\mu \hat{a}_\mu\rangle(t) = \frac{1}{2}\Big( \sum_\xi \left\{(\rho_{\rm b})_{\mu\xi,\mu\xi}(t) + [\phi_{\mu\xi}(t)]^2\right\} - 1\Big). \quad (25)$$

in two different regimes. The effective interaction strength is governed by $\gamma = g^2/(\omega T)$: intermediate coupling corresponds to $\gamma = 0.25$ (upper panel) and strong coupling to $\gamma = 1.0$ (lower panel).

The natural occupations are always zero and one at the mean-field level, as it should. The ***Gd*** approximation introduces correlation effects to some extent and approximates the exact solution well for short times. However, the envelope, more visible for $\gamma = 1.0$, is not captured. The ***GD*** approximation corrects for this deficiency. More importantly, the level of agreement between KBE and GKBA is of comparable quality.

The inadequacy of the ***Gd*** approximation is most evident in the boson number. Here ***Gd*** performs like mean-field and yields $\rho_{\rm b}(t) = \rho_{\rm b}(t_0)$, meaning $(\rho_{\rm b})_{11}(t) = (\rho_{\rm b})_{22}(t) = 1/2$. Thus, these approximations do not generate bosons, i.e., $\langle \hat{a}^\dagger \hat{a}\rangle(t) = 0$, a result which can be understood from Eq. (25) taking into account that $\phi_{1,2}(t) = 0$ by symmetry. The ***GD*** approximation considerably improves the situation both at the KBE and GKBA level, except for a slight underestimation and overestimation, respectively, in the strong coupling regime.

We remark that we find that for the ***GD*** approximation, the KBE solution damps, while the GKBA solution does not. This is consistent with findings in the electronic case.[14,15]

To test the stability of the GKBA, we time propagated until $t = 4000$ (100 times longer than in Fig. 1, not shown) without encountering any unphysical instability. To appreciate the computational gain, we report the approximate CPU time required for a ***GD*** run in the various schemes: $\sim$ 1 hour for the KBE, $\sim$ 1 minute for the integro-differential GKBA, and $< 1$ second for the ODE GKBA (the last two give identical results). We stress that our ODE implementation of the GKBA has the added advantage of being more numerically accurate, being fourth order, while the integro-differential schemes used are at most second order.[13,16]

### B. Energy conservation

In this section, we show an example how the conservation of energy is violated in the ***Gd*** approximation, which is not $\Phi$-derivable, but is maintained in the ***GD*** approximation, which is $\Phi$-derivable.

We choose our example to be the Holstein dimer with interaction strength $\gamma = 1.0$, and bosonic frequency $\omega = 0.1$. The dimer is driven out of equilibrium using the same protocol as in Sec. IV. Our results are shown in Fig. 2. For consistency, we use the definition of $E_c^{(1)}$ as correlation energy.

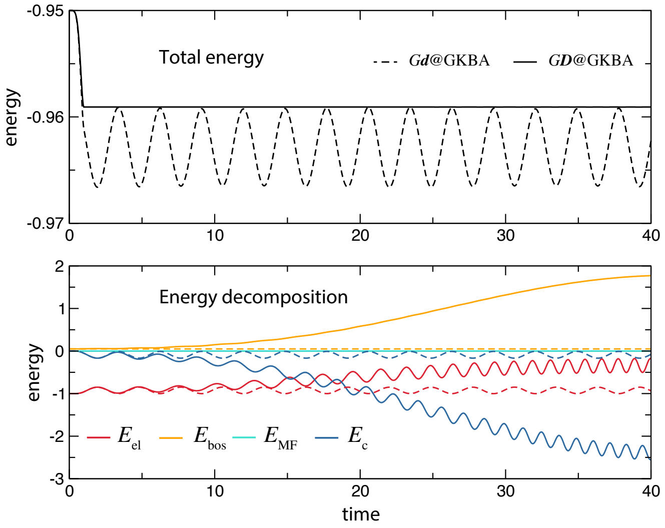


FIG. 2. Time-dependent energy for the Holstein dimer within the ***Gd*** (dashed lines) and ***GD*** (solid lines) approximations. ***GD*** is energy conserving, while ***Gd*** is not.

We first note that the mean-field contribution $E_{\rm MF} = 0$, as $\phi_{\bar{\mu}} = 0$. The free bosonic energy in the ***Gd*** approximation is $E_{\rm bos} = \omega/2$, constant in time, as the bosonic occupation number is zero. For the ***GD*** approximation, instead, the bosons can absorb energy from the electronic subsystem, and $E_{\rm bos}$ acquires a non-trivial time dependence. In the panel for the total energy, during the switching on of the interaction, the total energy changes. After the perturbation, we see that the total energy is not conserved in the ***Gd*** approximation, but is conserved for the ***GD*** approximation. We checked numerically that, for the ***Gd*** approximation, none of the definitions $E_c^{(1)}$, $E_c^{(2)}$ or $\frac{1}{2}(E_c^{(1)} + E_c^{(2)})$ of the correlation energy yields a conserved total energy.

## V. K-SPACE FORMULATION

In this section, we give the linear GKBA ODE scheme in $k$-space for a translationally homogeneous system. Quite generally, an electron index

$$i = (m, \alpha), \quad (26)$$

comprises the unit cell index $m$ and an extra degree of freedom $\alpha$ within the cell. Similarly, a boson index

$$\bar{\bar{\mu}} = (n, \bar{\mu}), \quad \bar{\mu} = (\mu, \xi), \quad (27)$$

is a composite index comprising the boson branch $\mu$ and the index $\xi = (1, 2)$ specifying the components of the boson field $\phi$, and $n$ is a cell index.

Invariance under discrete translations implies for the Hamil-

tonian ingredients

$$h^{(0)}_{i_1,i_2} = h^{(0)}_{\alpha_1\alpha_2}(m_1 - m_2), \tag{28a}$$
$$\Omega_{\bar{\mu}_1\bar{\mu}_2} = \Omega_{\bar{\mu}_1\bar{\mu}_2}(n_1 - n_2), \tag{28b}$$
$$\lambda^{\bar{\mu}_1}_{i_1 i_2} = \lambda^{\bar{\mu}_1}_{\alpha_1\alpha_2}(n_1 - m_1, n_1 - m_2). \tag{28c}$$

These conditions guarantee, that if a disturbance does not break translational invariance, then the bosonic field is independent of the cell index

$$\phi_{\bar{\bar{\mu}}_1} = \phi_{\bar{\mu}_1}(n_1) = \phi_{\bar{\mu}_1},$$

densities and scattering terms depend on the difference of cell indices

$$\rho_{i_1 i_2} = \rho_{\alpha_1\alpha_2}(m_1 - m_2), \qquad I_{i_1 i_2} = I_{\alpha_1\alpha_2}(m_1 - m_2),$$
$$\rho_{\mathrm{b}}^{\bar{\bar{\mu}}_1\bar{\bar{\mu}}_2} = \rho_{\mathrm{b}}^{\bar{\mu}_1\bar{\mu}_2}(n_1 - n_2), \qquad I_{\mathrm{b}}^{\bar{\bar{\mu}}_1\bar{\bar{\mu}}_2} = I_{\mathrm{b}}^{\bar{\mu}_1\bar{\mu}_2}(n_1 - n_2),$$

whereas two-body functions depend on the two differences of cell indices

$$\mathcal{G}^{\bar{\bar{\mu}}_1}_{i_1 i_2} = \mathcal{G}^{\bar{\mu}_1}_{\alpha_1\alpha_2}(n_1 - m_1, n_2 - m_2),$$
$$\Psi^{\bar{\bar{\mu}}_1}_{i_1 i_2} = \Psi^{\bar{\mu}_1}_{\alpha_1\alpha_2}(n_1 - m_1, n_2 - m_2).$$

Next we introduce the Fourier series for one-point functions

$$f(n_1 - n_2) = \frac{1}{N_k}\sum_{k_1} \mathrm{e}^{ik_1(n_1-n_2)} f(k_1),$$

and two-point functions

$$g(n_1 - n_2, n_1 - n_3) = \frac{1}{N_k^2}\sum_{k_1 k_2} \mathrm{e}^{ik_1(n_1-n_2)} g(k_1, k_2)\mathrm{e}^{-ik_2(n_1-n_3)},$$

where $N_k$ denotes the number of cells or, equivalently, the number of $k$-points.

With this we can write the linear ODE scheme for the *GD* approximation in $k$-space. In what follows, time-dependence is supressed, for ease of notation. We furthermore consider the *e-e* interaction in the mean-field approximation.

*a. Single-particle Hamiltonian*

$$h_{\alpha_1\alpha_2}(k) = h^{\mathrm{HF}}_{\alpha_1\alpha_2}(k) + h^{\mathrm{bos}}_{\alpha_1\alpha_2}(k), \tag{29}$$

where the Hartree-Fock Hamiltonian $h^{\mathrm{HF}}$ depends on the choice of the electron Hamiltonian that we do not specify here.

*b. Bosonic mean-field contribution*

$$h^{\mathrm{bos}}_{\alpha_1\alpha_2}(k) = \sum_{\bar{\mu}_1} \phi_{\bar{\mu}_1}\lambda^{\bar{\mu}_1}_{\alpha_1\alpha_2}(-k, -k). \tag{30}$$

*c. Bosonic $\phi$-field*

$$\left[i\boldsymbol{\alpha}\frac{\mathrm{d}}{\mathrm{d}t} - \bar{\boldsymbol{\Omega}}(k=0)\right]\boldsymbol{\phi} = \frac{1}{N_k}\sum_k\sum_{\alpha_1\alpha_2} \boldsymbol{\lambda}_{\alpha_1\alpha_2}(k,k)\rho_{\alpha_2\alpha_1}(-k). \tag{31}$$

*d. Equation of motion for the electronic density matrix*

$$\frac{\mathrm{d}}{\mathrm{d}t}\rho_{\alpha_1\alpha_2}(k) + i\sum_{\alpha_3}\left[h_{\alpha_1\alpha_3}(k)\rho_{\alpha_3\alpha_2}(k) - \rho_{\alpha_1\alpha_3}(k)h_{\alpha_3\alpha_2}(k)\right] = -I_{\alpha_1\alpha_2}(k) - I^*_{\alpha_2\alpha_1}(k). \tag{32}$$

*e. Equation of motion for the bosonic density matrix*

$$\frac{\mathrm{d}}{\mathrm{d}t}\boldsymbol{\rho}_{\mathrm{b}}(k) + i\left[\boldsymbol{\alpha}\bar{\boldsymbol{\Omega}}(k)\boldsymbol{\rho}_{\mathrm{b}}(k) - \boldsymbol{\rho}_{\mathrm{b}}(k)\bar{\boldsymbol{\Omega}}(k)\boldsymbol{\alpha}\right] = \boldsymbol{I}_{\mathrm{b}}(k) + \boldsymbol{I}^T_{\mathrm{b}}(-k). \tag{33}$$

*f. Electronic collision integral*

$$I_{\alpha_1\alpha_2}(k) = \frac{i}{N_k}\sum_{\bar{\mu}}\sum_{\alpha_3}\sum_p \lambda^{\bar{\mu}}_{\alpha_1\alpha_3}(-k,p)\mathcal{G}^{\bar{\mu}}_{\alpha_3\alpha_2}(p,-k). \tag{34}$$

*g. Bosonic collision integral*

$$I^{\bar{\mu}_1\bar{\mu}_2}_{\mathrm{b}}(k) = -\frac{i}{N_k}\sum_{\alpha_1\alpha_2}\sum_{\bar{\mu}_3}\sum_p \alpha_{\bar{\mu}_1\bar{\mu}_3}\lambda^{\bar{\mu}_3}_{\alpha_1\alpha_2}(p+k,p) \times \mathcal{G}^{\bar{\mu}_2}_{\alpha_2\alpha_1}(p,p+k). \tag{35}$$

*h. Equation for $\mathcal{G}$*

$$i\frac{\mathrm{d}}{\mathrm{d}t}\mathcal{G}^{\bar{\mu}_1}_{\alpha_1\alpha_2}(k_1,k_2) = \Psi^{\bar{\mu}_1}_{\alpha_1\alpha_2}(k_1,k_2) + \sum_{\bar{\mu}_2\bar{\mu}_3}\alpha_{\bar{\mu}_1\bar{\mu}_2}\Omega_{\bar{\mu}_2\bar{\mu}_3}(k_1-k_2) \times \mathcal{G}^{\bar{\mu}_3}_{\alpha_1\alpha_2}(k_1,k_2) + \sum_{\alpha_3}\Big[h_{\alpha_1\alpha_3}(-k_1)\mathcal{G}^{\bar{\mu}_1}_{\alpha_3\alpha_2}(k_1,k_2) - \mathcal{G}^{\bar{\mu}_1}_{\alpha_1\alpha_3}(k_1,k_2)h_{\alpha_3\alpha_2}(-k_2)\Big], \tag{36}$$

with $\boldsymbol{\Psi} = \boldsymbol{\Psi}^> - \boldsymbol{\Psi}^<$, and

$$\Psi^{\lessgtr\bar{\mu}_1}_{\alpha_1\alpha_2}(k_1,k_2) = \sum_{\bar{\mu}_2}\rho_{\mathrm{b}}^{\lessgtr\bar{\mu}_1\bar{\mu}_2}(k_1-k_2) \times \sum_{\alpha_3\alpha_4}\rho^{\lessgtr}_{\alpha_1\alpha_3}(-k_1)\lambda^{\bar{\mu}_2}_{\alpha_3\alpha_4}(k_1,k_2)\rho^{\gtrless}_{\alpha_4\alpha_2}(-k_2). \tag{37}$$

$\boldsymbol{I}$, $\mathcal{G}$ and $\boldsymbol{I}_{\mathrm{b}}$ are computationally the most time-consuming quantities. For a system with $N_{\mathrm{bands}}$ electron bands and $N_{\mathrm{branches}}$ phonon branches, we have $N_{\mathrm{e}} = N_{\mathrm{bands}}N_k$ and $N_{\mathrm{b}} = N_{\mathrm{branches}}N_k$. The $k$-space implementation reduces the computational scaling from $\mathcal{O}(N_{\mathrm{e}}^3 N_{\mathrm{b}})$ to $\mathcal{O}(N^3_{\mathrm{bands}}N_{\mathrm{branches}}N_k^2)$ for $I$, $\mathcal{G}$ and from $\mathcal{O}(N_{\mathrm{e}}^2 N_{\mathrm{b}}^3)$ to $\mathcal{O}(N^2_{\mathrm{bands}}N^3_{\mathrm{branches}}N_k^2)$ for $\boldsymbol{I}_{\mathrm{b}}$, respectively.

---

[1] Niko Säkkinen, Yang Peng, Heiko Appel, and Robert van Leeuwen, "Many-body Green's function theory for electron-phonon interactions: The Kadanoff-Baym approach to spectral

properties of the Holstein dimer," J. Chem. Phys. **143**, 234102 (2015).

[2] Niko Säkkinen, Yang Peng, Heiko Appel, and Robert van Leeuwen, "Many-body Green's function theory for electron-phonon interactions: Ground state properties of the Holstein dimer," J. Chem. Phys. **143**, 234101 (2015).

[3] Daniel Karlsson and Robert van Leeuwen, "Non-equilibrium Green's Functions for Coupled Fermion-Boson Systems," in *Handb. Mater. Model.*, edited by Andreoni W. and Yip S. (Springer International Publishing, Cham, 2018) pp. 1–29.

[4] Gordon Baym, "Self-Consistent Approximations in Many-Body Systems," Phys. Rev. **127**, 1391–1401 (1962).

[5] G. Stefanucci and R. van Leeuwen, *Nonequilibrium Many-Body Theory Quantum Syst. A Mod. Introd.* (Cambridge University Press, Cambridge, 2013).

[6] Niko Säkkinen, *Application of time-dependent many-body perturbation theory to excitation spectra of selected finite model systems*, Ph.D. thesis, University of Jyväskylä (2016).

[7] Miroslav Hopjan and Claudio Verdozzi, "Initial correlated states for the generalized Kadanoff–Baym Ansatz without adiabatic switching-on of interactions in closed systems," Eur. Phys. J. Spec. Top. **227**, 1939–1948 (2019).

[8] H. Mera, M. Lannoo, C. Li, N. Cavassilas, and M. Bescond, "Inelastic scattering in nanoscale devices: One-shot current-conserving lowest-order approximation," Phys. Rev. B **86**, 161404(R) (2012).

[9] I. V. Tokatly, "Conserving approximations in cavity quantum electrodynamics: Implications for density functional theory of electron-photon systems," Phys. Rev. B **98**, 235123 (2018).

[10] Jozef T. Devreese and Alexandre S. Alexandrov, "Fröhlich polaron and bipolaron: recent developments," Reports Prog. Phys. **72**, 066501 (2009).

[11] Phillip Weinberg and Marin Bukov, "QuSpin: a Python package for dynamics and exact diagonalisation of quantum many body systems part I: spin chains," SciPost Phys. **2**, 003 (2017).

[12] Phillip Weinberg and Marin Bukov, "QuSpin: a Python package for dynamics and exact diagonalisation of quantum many body systems. Part II: bosons, fermions and higher spins," SciPost Phys. **7**, 020 (2019).

[13] M. Schüler, J. Berakdar, and Y. Pavlyukh, "Time-dependent many-body treatment of electron-boson dynamics: Application to plasmon-accompanied photoemission," Phys. Rev. B **93**, 054303 (2016).

[14] Marc Puig von Friesen, C. Verdozzi, and C.-O. Almbladh, "Kadanoff-Baym dynamics of Hubbard clusters: Performance of many-body schemes, correlation-induced damping and multiple steady and quasi-steady states," Phys. Rev. B **82**, 155108 (2010).

[15] Sebastian Hermanns, Niclas Schlünzen, and Michael Bonitz, "Hubbard nanoclusters far from equilibrium," Phys. Rev. B **90**, 125111 (2014).

[16] Enrico Perfetto and Gianluca Stefanucci, "CHEERS: a tool for correlated hole-electron evolution from real-time simulations," J. Phys. Condens. Matter **30**, 465901 (2018).
